# Supplementary material for: Coarser Equivalences for Causal Concurrency
Source: arXiv:2208.12117 source file (2023-10-26)
Supplement: Supplementary file 1 [file appendix-blocks.tex]

% !TEX root = main.tex
\section{Proofs of Theorems in Section \ref{sec:bpo}}

\subsection{Proof of The Completeness Theorem \ref{thm:coincidence}}

\begin{proof}
The $\Rightarrow$ direction is Lemma \ref{lem:lin-eq}. For the other direction, we rely on a lemma that is stated and proved after the completion of this proof. 

We prove the $\Leftarrow$ direction by showing that we can {\em bubble sort} $u$ to get $v$, using the two types of swaps that are outlined in Definition \ref{def:beq}, limited to blocks in $\blocks$. Starting from the index $0$, we identify the location of the next $v[i]$ in $u$ and swap it backwards to position $i$. Formally, we prove by induction that for all index $i$, $v[i]$ can be successfully placed after $v[0] \dots v[i-1]$ have been placed, to produce an intermediate string $v'$ where $v' \fbeq u$ and $v' \bleq u$.

Base Case: Let $i = 0$. Let $v[0] = e$ and $u = \alpha e \beta$. By definition of $\bhb$ and the fact that $v \bleq u$, using Lemma \ref{lem:scope}, we argue that $e$ can be swapped back to the beginning of the word resulting in a word $u' = e \sigma$.  By Lemma \ref{lem:lin-eq}, we also have $u' \bleq u$.

The Induction Hypothesis: Let us assume we can place the first $n - 1$ symbols of $v$ through swaps. Let $\alpha$ be the prefix of $v$ of length $n - 1$. Let $w = \alpha \beta e \sigma$. We know that  $w \fbeq u$, $\blocks$ are valid liberally atomic blocks of $w$,  and $w$ is a proper linearization of $\bhb$.

The goal is to show that we can swap $e = v[n]$ into place and satisfy the induction hypothesis. As before, since $v$ is a proper linearization of $\bhb$ and $e$ appears at the position $n$ of $v$, then by Lemma \ref{lem:scope}, $e$ can be swapped back to position $n$. The resulting string $u'$ will satisfy $u' \bleq w$ and is a proper linearization of $\bhb$.  
\end{proof}

\begin{lemma}[Scope]\label{lem:scope}
Consider a word $u$ and fix a set of liberally atomic blocks $\blocks$ for $u$ which induces the partial order $\bhb$. Let $u = v w e w'$ and assume that $vev'$ is a proper linearization of $\bhb$. Then, $u \fbeq vev'$.
\end{lemma}
%%%

\begin{proof}
Observe that by the definition of a proper linearization, no event $f$ in $w$ can satisfy $f \bhb e$. Therefore, no event $f$ in $w$ can share a thread with $e$. We show that $e$ can be swapped backwards in $w$ until it reaches the beginning of $w$ as follows. In each case, we also argue that, after each step, the resulting word $u'$ satisfies $u \fbeq u'$.
\begin{itemize}
\item[(i)] If $w$ only contains events that access a variable other than $\VariableOf{e}$, and considering that no event in $w$ can share a thread with $e$, we can conclude that $e$ does commute against every event in $w$ in the classic trace thoery sense. Therefore, $v w e w' \meq v e w w'$. By Theorem \ref{thm:hierarchy}, we can conclude that $vwew' \fbeq veww'$.
%Besides, all the single event swaps, by Lemma \ref{lem:maz-lin}, preserve $\bleq$.

\item[(ii)] If $w$ contains events $f$ such that $\VariableOf{f} = \VariableOf{e}$, then by the definition of $\bhb$,  $e$ and all such $f$'s must be part of some blocks in $\blocks$, or we would arrive at the contradiction $f \bhb e$. There are two possibilities for the location of $e$ in its block $B_e$. If is not the first event, then another event $e'$ is the first event of $B_e$ and we have $e' \bhb e$. Therefore, $e'$ cannot be in $w$. But, it must have appeared before $e$ in $u$, and therefore it must be in $v$. But then, by definition of blocks, all events accessing $\VariableOf{e}$ in $w$ must belong to $B_e$ as well; since blocks over the same variable cannot overlap. Since these are all read events and none of them can share a thread with $e$, this case defaults back to case (i) where $e$ can be swapped back over all such events in the classic trace theory sense, and $v e w v'\meq v w e v'$. 

Let us now consider the case that $e$ is the first event of $B_e$. We argue using the following steps:
\begin{itemize} 
    \item Since in $vwew'$ no two blocks over the same variable overlap, we can conclude that all events $f$ over the $\VariableOf{e}$ in $w$ are part of blocks that begin and end in $w$. If not, one such block would begin in $v$ and end in $w$, and that is a contradiction against the existence of a proper linearization in the form of $vev'$.
	\item By the definition of liberally atomic blocks, we know there exists a word $\sigma \fbeq wew'$ such that the block of $e$ and all events $f$ in $w$ that access $\VariableOf{v}$ appear serially in $\sigma$. Note that if a set of blocks $\blocks$ is liberally atomic, then any subset of it is also by definition liberally atomic. Since $v \sigma \fbeq vwew'$, by Lemma \ref{lem:lin-eq}, we also have $v \sigma \bleq vwew'$. Therefore, in its new position in $v\sigma$, $e$ still respects the constraints of $\bhb$. 
	\item In $v \sigma$, we argue that $B_e$ can be swapped back to the beginning of $\sigma$. Everything on its way is either an independent event accessing another variable in another thread or a block accessing $\VariableOf{v}$. Moreover, for each such block $B$, we know $\ThreadsOf{B} \cap \{\ThreadOf{e}\} = \emptyset$. If not, then the assumption of the lemma would be violated. It remains to argue that $\ThreadsOf{B} \cap \ThreadsOf{B_e} = \emptyset$. Let us assume this is not true. We argue that there cannot exist a $v'$ such that $vev'$ is a proper linearization of $\bhb$. If $vev'$ is a proper linearization, then any such block $B$ has to appear in $v'$ after the last event of $B_e$. Then, by definition, $vev'$ cannot be a linearization of $\bhb$ which includes $PO$ edges that are broken in $vev'$. 
	  
	We can conclude that $B_e$ can then be commuted back,  resulting in a word $v B_e \sigma'$ which clearly satisfies $v B_e \sigma' \fbeq v\sigma \fbeq vwew'$.

\end{itemize}
\end{itemize}

\end{proof}

\subsection{Proof of The Proper Topological Sorting Theorem \ref{thm:tsort}}

\begin{proof}
Observe that the algorithm clearly maintains an invariant that $v$ never violates the condition of being a proper linearization of the set of events in $E$. It is rather straightforward then that if the algorithm does not get stuck on step (2), what it produces is a proper linearization by definition. Therefore, the only interesting part of this argument is to show that while $E \neq \emptyset$, step (2) always succeeds at finding an event $e$ satisfying the constraints.

Let us assume the opposite. Since $\bhbs$ is a partial order, there is always an event $e$ satisfying the first condition ($\not \exists f \in E:\ f \bhbs e$). The only possibility is that any such event will force an overlap of blocks of the same variable. We argue that this cannot happen. Consider an arbitrary open block $B$. Let $S$ be the set of all such events that satisfy the first condition, but not the second one. The following statements are true about $S$:
\begin{itemize}
\item None of the remaining events of any such $B$ can belong to $S$. 
\item No event in $S$ can be a stand alone event (not part of any block).
\end{itemize}
This leaves us only with the option that all events in $S$ are the start of a new block which shares a variable with an open block $B$. Moreover, for each remaining event $f$ of any such block $B$, there is an event $f' \in S$ such that $f' \bhbs f$. The part that some dependency to an event not yet scheduled in $v$ is causing $f$ not to be in $E$ is clear. If a missing event like this is itself not in $E$, then recursively, it must have predecessor in $E$. 

Note that $f'$ cannot share a variable with $f$. This causes a contradiction to the definition of $\bhbs$. So, we establish that the remaining of every block open on some variable $x$ cannot belong to $E$ due to a dependency on some other open block on variable $y$. This forms a permutation over blocks, with no identities, which is well-understood to include a cycle of size 2 or more. This cycle witnesses that the blocks involved cannot be liberally atomic. Hence a contradiction.
\end{proof}

\subsection{Proof of The Soundness Theorem \ref{thm:soundness}}

\begin{proof}
First, observe that the following statement is true in a straightforward manner:
if $e \bhb e'$ then there does not exist a word $v \fbeq u$ in which $e'$ appears before $e$.

$\implies$ direction: If $e \bhb e'$, we have nothing to prove. Therefore, we assume $e \not \bhb e'$ and yet $e \bhbs e'$. Let us consider the shortest chain from $e$ to $e'$ to be $e \bhbs f_1 \dots \bhbs f_k \bhbs e'$. We prove our goal by induction on $k$. If $k = 0$, then the only possibility is that $e \bhbs e'$ is introduced through one application of the  saturation rule \ref{rule3}, from which we can conclude the order cannot be flipped. Assume this is true for $k - 1$ intermediate events, and we prove it for $k$. The statement is by induction through for the pair of events $(e, f_k)$ and also for the pair $(f_k, e')$. If $(e,e')$ can be reordered in another proper linearization, then in that at least one of these pairs must be reordered as well, which is a contradiction.

$\Longleftarrow$ direction: Assume that $e \not \bhbs e'$.  We prove that there exists a word $v \fbeq u$ in which $e'$ appears before $e$. We prove this using the strong scope lemma. Let $u = w e w' e' w''$. A few important straightforward observations:
\begin{itemize}
\item For any event $f \in w'$ where $f \bhbs e'$, we have $e \not \bhbs f$.
\item If $f,f' \in w'$ and $f \bhbs e'$ and $f' \not \bhbs e'$, then $f' \not \bhbs f$.
\item The set of events that satisfy $e \bhbs f$ is disjoint from the set of events that satisfy $f \bhbs e'$.
\end{itemize}

Consider the following set of simple rules, and let $E$ be the smallest set of events that is closed under these rules:
\begin{align}
&e' \in E \\
f \bhbs e' \implies &f \in E \\
f \in B_g \wedge g \in E \implies &g \in E
\end{align}
Observe that $e \not \in E$. We argue that there is a proper linearization $v$ that starts with a proper linearization of events in $E$, followed by $e$, and then followed by whatever is left of $u$. This is done through Theorem \ref{thm:tsort}. We use the algorithm presented in it to do a proper linearization of $E$, which does not include $e$, and then continue with the algorithm to completion where $e$ is bound to appear somewhere later. 
\end{proof}

\subsection{Proof of The Scope Theorem}

\begin{proof}
The proof is straightforward, given Theorem \ref{thm:tsort}. We can start the algorithm in the theorem from the point at the end of $v$ (rather than $\epsilon$), with all the open blocks from $v$ considered as open. We let $E$ be the set of events in $wew'$. Since no event $f$ that appears after $e$ in $u$ can satisfy $f \bhbs e$ by definition, and no such events exist in $w$, they all must be in $v$. Then $e$ will satisfy both conditions in step (2) of the proper topological sorting algorithm, and can be selected to be scheduled after $v$. The algorithm then continues to completion and produces a proper linearization. 
\end{proof}

%%%

Alternative Proof:

\begin{proof}
Since there is no event $f$ in $w$ can satisfy $f \bhbs e$, and $u$ is a proper linearization, we can conclude that any event $f$ such that $f \bhbs e$ belongs to $v$. We show that $e$ can be swapped backwards in $w$ until it reaches the beginning of $w$ as follows. 
\begin{itemize}
\item[(i)] If $e$ is an event that does not belong any block, then this case defaults to a simple argument for why $u \meq veww'$, and therefore, we can let $v' = ww'$ and conclude that $vev'$ is a proper linearization of $\bhbs$. 
\item[(ii)] If $e$ does belong to a block, then the only option for it is to be the first event of that block.  

If $w$ contains events $f$ such that $\VariableOf{f} = \VariableOf{e}$, then by the definition of $\bhb$,  all such $f$'s must be part of some blocks in $\blocks$, or we would arrive at the contradiction $f \bhb e$. The difference between our argument here, and that of the original scope lemma is that we have weaker assumptions to utilize. In particular, we argue that $e$ can be swapped back, but we cannot make the same argument about $B_e$ (the block of $e$) as a whole. There may be events in $w$ that permit $e$ alone to be swapped back, but not the rest of its block. 

We argue using the following steps:
\begin{itemize} 
    \item Since in $vwew'$ no two blocks over the same variable overlap, we can conclude that all events $f$ over the $\VariableOf{e}$ in $w$ are part of blocks that begin and end in $w$. If not, one such block would begin in $v$ and end in $w$, and that is a contradiction against the existence of a proper linearization in the form of $vev'$.
	\item By the definition of liberally atomic blocks, we know there exists a word $\sigma \fbeq wew'$ such that the block of $e$ and all events $f$ in $w$ that access $\VariableOf{e}$ appear serially in $\sigma$. Note that if a set of blocks $\blocks$ is liberally atomic, then any subset of it is also by definition liberally atomic. Since $v \sigma \fbeq vwew'$, by Lemma \ref{lem:lin-eq}, we also have $v \sigma \bleq vwew'$. Therefore, in its new position in $v\sigma$, $e$ still respects the constraints of $\bhb$. 
	\item In $v \sigma$, we argue that $B_e$ can be swapped back against all other blocks that access $\VariableOf{e}$, but necessarily all the way to the beginning of $\sigma$. After this is done, we argue that $e$ can be swapped the rest of the way back in $\sigma$ alone.

	Let us first focus on the blocks that we serialized in $\sigma$. For each such block $B$, we know $\ThreadsOf{B} \cap \{\ThreadOf{e}\} = \emptyset$. If not, then the assumption of the lemma would be violated. It remains to argue that $\ThreadsOf{B} \cap \ThreadsOf{B_e} = \emptyset$. Let us assume this is not true. Then by definition of $\bhbs$, we will have every event $f$ in such a block $B$ to satisfy $f \bhbs e$, which is a contradiction. Therefore, $B_e$ is swappable against all such blocks $B$. 
	
	Now let us focus on all other $f$ events in $\sigma$ that satisfy $\VariableOf{e} \neq \VariableOf{f}$. Any such event $f$ that does not satisfy $\exists e' \in B_e:\ f \bhbs e'$ can be swapped against all of $B_e$ using the classic independent event swaps, and therefore does not pose an obstacle. So, we focus on those that satisfy the constraint. The key observation is that any such event $f$ can {\em join} $B_e$ and be swapped backward with it against all other $B$ blocks mentioned above. If not, then $f$ witnesses a dependency between a block $B$ and $B_e$ and produces a contradiction. 
	
	Once $B_e$ collects all such event $f$ and moves backwards against all blocks $B$, then $e$ separates from its block $B_e$ and swaps back against all collected and remaining events $f$ in $w$.  
\end{itemize}
\end{itemize}

\end{proof}
